# Supplementary material for: Multi-level Explanation of Deep Reinforcement Learning-based Scheduling
Source: arXiv:2209.09645 source file (2022-09-18)
Supplement: Supplementary file 1 [file Section_8_appendix.tex]

\section{Training of Decima.}
The DRL-based scheduler Decima is trained under the following settings. Totally, 100 streamed TPC-H jobs come in based on the Poisson process, with time interval of 25 seconds. The reward function is set to optimize average job completion time, and calculated by minimizing $\mathbb{E}\left [ 1/t_T {\textstyle \sum_{k=1}^{T}(t_k-t_{k-1})J_k}  \right ] $, where $J_k$ is the number of jobs in system during time interval $[t_{k-1}, t_k)$ \cite{mao19learning}. The learning rate is set to 0.001 and the Adam optimizer is used. The policy is learned with 8 parallel agents, of which the retrieved rewards are averaged for policy improvement. The training process is shown in Figure~\ref{fig:training_curve}. The code of Decima and its integration with our explanation framework is open sourced \footnote{The repository is https://github.com/zhangsj0608/decima-sim.git.}.   

\begin{figure}[htbp]
    \centering
    \includegraphics[width=0.45\linewidth]{Figures/training_curve.pdf}
    \caption{The training process of Decima.}
    \label{fig:training_curve}
\end{figure}

\section{Additional examples on fine-tuned job choices} 
Different trees in the random forest model have varied structure, but often give unified explanation towards the job choices through their decision paths. We give an additional example to show how the paired jobs are compared by multiple trees. The job features are listed in Table~\ref{tab: job-features-concate}, and $Job_i$ is scheduled for execution at the specific schedule time step. Notice, the features are indexed from 0 to 5, which are in regarding to explainable features (1) to (6) respectively.

The decision paths through 5 trees are shown in Figure~\ref{fig:tree-paths-appendix}. Each tree gives same classification results, in which $Job_i$ is scheduled rather than $Job_k$. We have the following observations: (i) different trees give similar patterns in deciding which job is more likely to be scheduled, by mainly focusing on specific features such as remaining run time ($Feature~4$) and task numbers ($Feature~5$) of the smallest ready node. (ii) the thresholds to split the nodes on the same feature across different trees are also similar. For example, the second nodes of $Tree_1, Tree_3, Tree_4, \mbox{and}~Tree_5$ share the quite similar or same thresholds on $Feature~5$ of $Job_k$. (iii) the explanation of job choice can be derived from the comparison of the same feature on the paired jobs. Hence, the explanations of job choice though different trees are coherent. 

%same paired job at different tree
\begin{table}[h]
\centering
\caption{The job features to be concatenated and classified through RF model.}
\begin{tabular}{ccccccc}
\hline
Feature      & 0       & 1    & 2       & 3    & 4     & 5   \\ \hline
$Job_i(scheduled)$ & 112.44  & 614  & 115.88  & 616  & 4.62  & 2   \\
$Job_k$ & 1385.17 & 1080 & 1600.87 & 1186 & 215.7 & 580 \\ \hline
\end{tabular}
\label{tab: job-features-concate}
\end{table}

\begin{figure}[t]
    \centering
    \includegraphics[width=0.98\linewidth]{Figures/nips-appendix-tree-paths.pdf}
    \caption{The decision paths in 5 different trees of the random forest model to classify which job should be scheduled. Tree nodes in regarding to $Job_i$ are shaded blue, while those for $Job_j$ are shaded green. The threshold of job feature (Feat.) is included in each node. Job features are included in Table~\ref{tab: job-features-concate}}
    \label{fig:tree-paths-appendix}
\end{figure}

% same chosen job with different paired job 

\section{Additional job perturbation examples}
We provide more examples on different node-split job perturbations to illustrate the power of the perturbation after knowing how the DRL-based scheduler operates.  Recall, Decima prefers jobs with small ready nodes. We explore the vulnerability by splitting task node into multiple smaller nodes. Basically, we carried out 3 node-split plans on the same job, as shown in Figure~\ref{fig:node-split-plan-1} and \ref{fig:node-split-plan-2}. As shown by Figure~\ref{fig:node-split-plan-1}, the original $Node~0$ contains 29 homogeneous tasks, and in Plan 1 it is split into two smaller nodes, containing 28 and 1 tasks respectively. As shown in Figure~\ref{fig:node-split-plan-2}, in Plan 2, it is split to 5 nodes, of which one contains 25 tasks and each of the others contains 1 task. In plan 3, which is an extreme case, it is split to 9 nodes, of which one contains 21 tasks and each of the others contains 1 task. The perturbed jobs are executed with the same amount of background jobs respectively, and the completion time are shown in Table~\ref{tab:jct-multi-perturbation-plans}. The perturbed job in node-split Plan 3 ( the best plan) achieves 33.2\% decrease on completion time comparing to the original job.
Here we have the following observation: if a task node is split into more smaller nodes, it can be completed faster by more powerful preemption of computation resources. This phenomena should be paid more attention to by the cluster administrator, when the DRL-based job scheduler is adopted in real-world cloud datacenters.

\begin{figure}[t]
    \centering
    \includegraphics[width=0.75\linewidth]{Figures/nips-split-plan-appendix-1.pdf}
    \caption{The original job DAG (left-hand) and node-split Plan 1 (right-hand). In Plan 1, $Node~0$ (in shaded color), which contains 29 tasks originally, is split to two nodes, containing 1 and 28 tasks respectively. The node containing the majority of tasks is shaded dark green.}
    \label{fig:node-split-plan-1}
\end{figure}

\begin{table}[h]
\centering
\caption{Completion time (JCT) of perturbed jobs when executed with same background jobs. The original job without perturbation is noted as 'w/o'. }
\begin{tabular}{ccccc}
\hline
Perturbation & w/o & Plan 1 & Plan 2 & Plan 3 \\ \hline
JCT & 223.615 & 222.163 & 215.989 & 149.09 (best) \\ \hline
\end{tabular}
\label{tab:jct-multi-perturbation-plans}
\end{table}

\begin{figure}[t]
    \centering
    \includegraphics[width=0.85\linewidth]{Figures/nips-split-plan-appendix-2.pdf}
    \caption{The node-split Plan 2 (left-hand) and node-split Plan 3 (right-hand). In Plan 2, $Node~0$ is split to five nodes. The larger one contains 25 tasks (in dark green), while the other 4 contain 1 task each. In Plan 3, $Node~0$ is split to 9 nodes. The larger one contains 21 tasks, while the others contain 1 task each. }
    \label{fig:node-split-plan-2}
\end{figure}
